# Supplementary material for: Semi-stochastic full configuration interaction quantum Monte Carlo: developments and application
Source: arXiv:1502.04847 ancillary file (2015-04-29)
Supplement: Supplementary file 1 [file supp_material.pdf]

# Supplemental material for "Semi-stochastic full configuration interaction quantum Monte Carlo: developments and application"


N. S. Blunt,[1,a)] Simon D. Smart,[2] J. A. F. Kersten,[1] J. S. Spencer,[3,4] George H. Booth,[1,5] and Ali Alavi[1,2]

[1)] *University Chemical Laboratory, Lensfield Road, Cambridge, CB2 1EW, U.K.*

[2)] *Max Planck Institute for Solid State Research, Heisenbergstraße 1, 70569 Stuttgart, Germany*

[3)] *Department of Materials, Imperial College London, Exhibition Road, London, SW7 2AZ, U.K.*

[4)] *Department of Physics, Imperial College London, Exhibition Road, London, SW7 2AZ, U.K.*

[5)] *Department of Physics, King's College London, Strand, London WC2R 2LS, U.K.*


## I. THE INITIATOR APPROXIMATION

In the initiator approximation to FCIQMC (i-FCIQMC), walkers whose weight exceeds a predetermined cutoff, $n_a$, are labeled "initiators". The spawning in i-FCIQMC, relative to full FCIQMC, is modified as follows: All spawnings from initiators survive as usual. All spawnings to sites occupied on the previous iteration also survive. However, spawnings from non-initiators to unoccupied sites only survive if there is at least one more spawning to the same site with the same sign. This adaptation removes the unmanageable noise found at small walker populations in the full scheme. Instead, it introduces an error in the sampled estimates, which is systematically reducible by increasing the walker population. It has allowed significantly larger systems to be studied than would be possible without the approximation.

This adaptation clashes somewhat with the semi-stochastic adaptation where all projection needs to be performed exactly within the deterministic space. In their semi-stochastic adaptation to i-FCIQMC, Petruzielo *et al.*[1] let the initiator cutoff, $n_a$, vary so that

$$n_a = cm^p \tag{1}$$

where $c$ and $p$ are constants (which they set to 1) and $m$ is the number of moves since the walker last visited the deterministic space.

In this work a simpler modification is used. We simply let all deterministic states be initiators (which is also enforced by the scheme used in Ref. (1)). We find this approach preferable since it is simpler both conceptually and in code. In figure 1, figure 4 from Ref. (1) is reproduced with these simpler rules. It is seen that the same benefit occurs.

Although we have not performed a comprehensive study of how semi-stochastic alters the initiator error, we have usually found that it does not make a significant difference in the cases we have studied. In particular this is observed when the number of walkers is much greater than the size of the deterministic space. This is expected, as in this limit the initiator approximation in both methods will become identical.

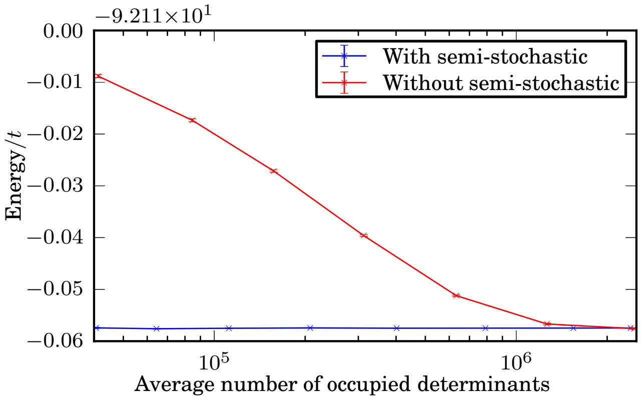


FIG. 1. Results showing the initiator error with and without the semi-stochastic adaptation, for the Hubbard model at $U/t = 1$ on an $8 \times 8$ square lattice, with 50 electrons. The deterministic space consists of the 16540 states connected to the Hartree–Fock state. This is a repeat of the results presented by Petruzielo *et al.*[1], but without the use of their graduated adaptation to the initiator rules. Instead the only adaptation to the standard initiator rules is that all deterministic states are forced to be initiators. The same reduction in initiator error observed by Petruzielo *et al.* is also observed with this simpler initiator scheme.

Interestingly, it is sometimes observed that the use of semi-stochastic can change the convergence of the initiator error. This is seen in figure 2, where $N_2$ is studied in a cc-pVDZ basis with 4 core electrons uncorrelated and at equilibrium geometry ($2.118a_0$). When using a deterministic space of up to and including two excitations from the Hartree–Fock state, convergence occurs from below the exact ground-state energy. This is potentially surprising because one might expect a CISD space to contain more highly weighted states at equilibrium geometry than a CAS space, which is seen to not alter the initiator error so significantly.


[a)] Electronic mail: nsb37@cam.ac.uk

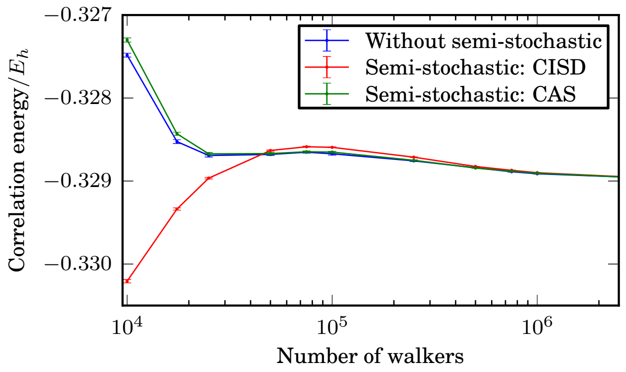


FIG. 2. Results showing the initiator error without the semi-stochastic adaptation, and with the adaptation and two different deterministic spaces. The system is $N_2$ in the cc-pVDZ basis, with 4 core electrons uncorrelated, and at equilibrium geometry ($2.118a_0$). Time-reversal symmetrized basis states[2] were used. The red curve shows results with a deterministic space of up to and including double excitations of the Hartree–Fock (1098 states). The green curve shows results where the deterministic space is a CAS (6,7) space (984 states), chosen for its similar size to the CISD space. Interestingly, the CISD result converges from below the exact energy.

## II. HOMOGENEOUS ELECTRON GAS RESULTS

In addition to the Hubbard and molecular systems studied, we have considered the usefulness of semi-stochastic for the homogeneous electron gas. FCIQMC has previously been used to study this system in detail[3–5]. Here we consider the 14-electron gas with 114 spin orbitals as the density parameter, $r_s$, is varied.

Figure 3 shows results for the Hartree–Fock energy estimator, as $r_s$ is varied from 0.5 a.u. to 4 a.u. Significant improvements in stochastic efficiency are seen. Once again it is found that less multi-configurational systems (low $r_s$) receive a greater benefit from the use of semi-stochastic. A slight decrease in stochastic efficiency is seen from $|D| = 10^4$ to $|D| = 10^5$ for $r_s = 4$ a.u. This is due to an increase in simulation time. As is found for simulations on the Hubbard model, the simulation time is reduced for systems dominated by a small number of states (primarily due an improvement of balancing of work among processors), and increased slightly for very multi-configurational systems.

In figure 4 we consider the relative efficiency for RDM estimates of $\langle S^2 \rangle$, calculated using the procedure in the main text, for values of $r_s$ from 0.25 a.u. to 4 a.u. Once again significant improvements occur with semi-stochastic, although a decrease in stochastic efficiency occurs from $|D| = 10^4$ to $|D| = 10^5$ for $r_s = 2$ a.u. and $r_s = 4$ a.u., once again due to an increase in simulation time. We therefore suggest that such large spaces are not sensible in very multi-configurational systems.

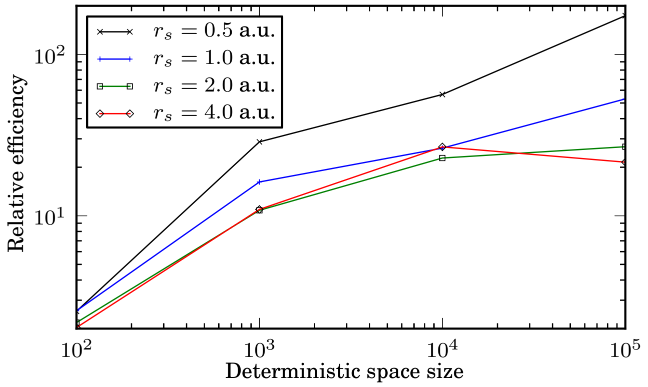


FIG. 3. The efficiency ($\epsilon_{E_0}$) of semi-stochastic simulations relative to an otherwise identical simulation without semi-stochastic, for the homogeneous electron gas with 14 electrons and 114 spin orbitals. As for the Hubbard model as $U/t$ is varied, it is found that semi-stochastic helps more at low $r_s$, where the wave function is more single-reference in nature. However, the benefit (and range of benefits) is not so large here as for the equivalent Hubbard model plot.

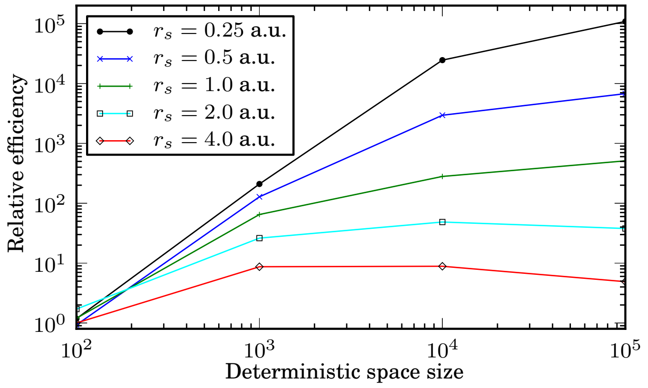


FIG. 4. The efficiency ($\epsilon_{\langle S^2 \rangle}$) of semi-stochastic simulations relative to an otherwise identical simulation without semi-stochastic, for the homogeneous electron gas with 14 electrons and 114 spin orbitals. This efficiency measure uses the estimate of $\langle S^2 \rangle$ obtained from stochastically-sampled RDMs. In common with the results based on the Hartree–Fock energy estimator (figure 3), a greater benefit is found for small $r_s$, although a significant improvement is found in all cases.


[1] F. R. Petruzielo, A. A. Holmes, H. J. Changlani, M. P. Nightingale, and C. J. Umrigar, Phys. Rev. Lett. **109**, 230201 (2012).
[2] S. Y. G. and L. Doreste-Suarez, Int. J. Quantum Chem. **7**, 687 (1973).
[3] J. J. Shepherd, G. H. Booth, A. Grüneis, and A. Alavi, Phys. Rev. B **85**, 081103(R) (2012).
[4] J. J. Shepherd, G. H. Booth, and A. Alavi, J. Chem. Phys. **136**, 244101 (2012).
[5] J. J. Shepherd, A. Grüneis, G. H. Booth, G. Kresse, and A. Alavi, Phys. Rev. B **86**, 035111 (2012).
